# Supplementary material for: Sulfur and sulfur-oxide compounds as potential optically active defects on SWCNTs
Source: arXiv:2409.18283 source file (2025-12-16)
Supplement: Supplementary file 1 [file SupportingInfo.pdf]

# Supporting Information for “Sulfur and sulfur-oxide compounds as potential optically active defects on SWCNTs”

Tina N Mihm,<sup>†</sup> Kasidet Jing Trerayapiwat,<sup>‡</sup> Xinxin Li,<sup>‡</sup> Xuedan Ma,<sup>‡</sup> and Sahar Sharifzadeh<sup>\*,†</sup>

<sup>†</sup>*Department of Electrical and Computer Engineering, Boston University, MA, 02215, USA*

<sup>‡</sup>*Center for Nanoscale Materials, Argonne National Laboratory, Lemont, IL 60439, USA*

<sup>¶</sup>*Consortium for Advanced Science and Engineering, University of Chicago, Chicago, IL 60637, USA*

<sup>§</sup>*Materials Science and NanoEngineering, Rice University, Houston, TX, 77251, USA*

<sup>||</sup>*Northwestern Argonne Institute of Science and Engineering, Evanston, IL 60208, USA*

<sup>⊥</sup>*Department of Chemistry, Boston University, Boston, MA, 02215, USA*

<sup>#</sup>*Materials Science Division, Boston University, Boston, MA, 02215, USA*

<sup>@</sup>*Department of Physics, Boston University, Boston, MA, 02215, USA*

E-mail: [ssharifz@bu.edu](mailto:ssharifz@bu.edu)

## 1 Experimental photoluminescence spectrum of SO<sub>x</sub>-defective (6,5) SWCNT

Figure [S.1](#) presents the raw photoluminescence data. Data in the main text was normalized by taking the max value of the largest peak and dividing all data by this emissions value.

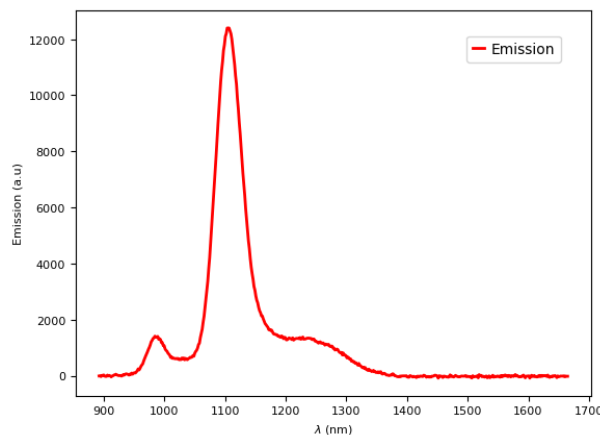

Figure S.1: Photoluminescence spectrum of (6,5) SWCNT after exposure to sodium dodecyl sulfate.

## 2 Binding information for $\text{SO}_x$ adsorbates

### 2.1 Unbound structures considered

In addition to the binding described in the main text, we tested additional structures for SO and  $\text{SO}_3$  that were found to be unbound and therefore not presented. For the SO molecule, epoxide-type binding was considered in addition to structure 3 of Figure 2(a) of the main text. For  $\text{SO}_3$ , in addition to the flat-type binding shown in Figure 2(a) of the main text, we tested an OO-loop-type binding and ether-type binding where the  $\text{SO}_3$  binds onto the 1, 3 carbons in the hollow site.

### 2.2 Detailed binding energies and charge transfer

Table S.1 presents detailed bonding information for the seven adsorbates presented in the manuscript, including bond angles, bond lengths and distance from the SWCNT surface. The bond angles for the  $\text{SO}_2$  and  $\text{SO}_3$  molecules are also shown in the table.

### 2.3 Charge transfer between molecule and adsorbate

Figure S.2 presents the calculated charge density differences for the five defect systems shown in Figure 4 in the main text. For S and SO, there is charge sharing between the adsorbate

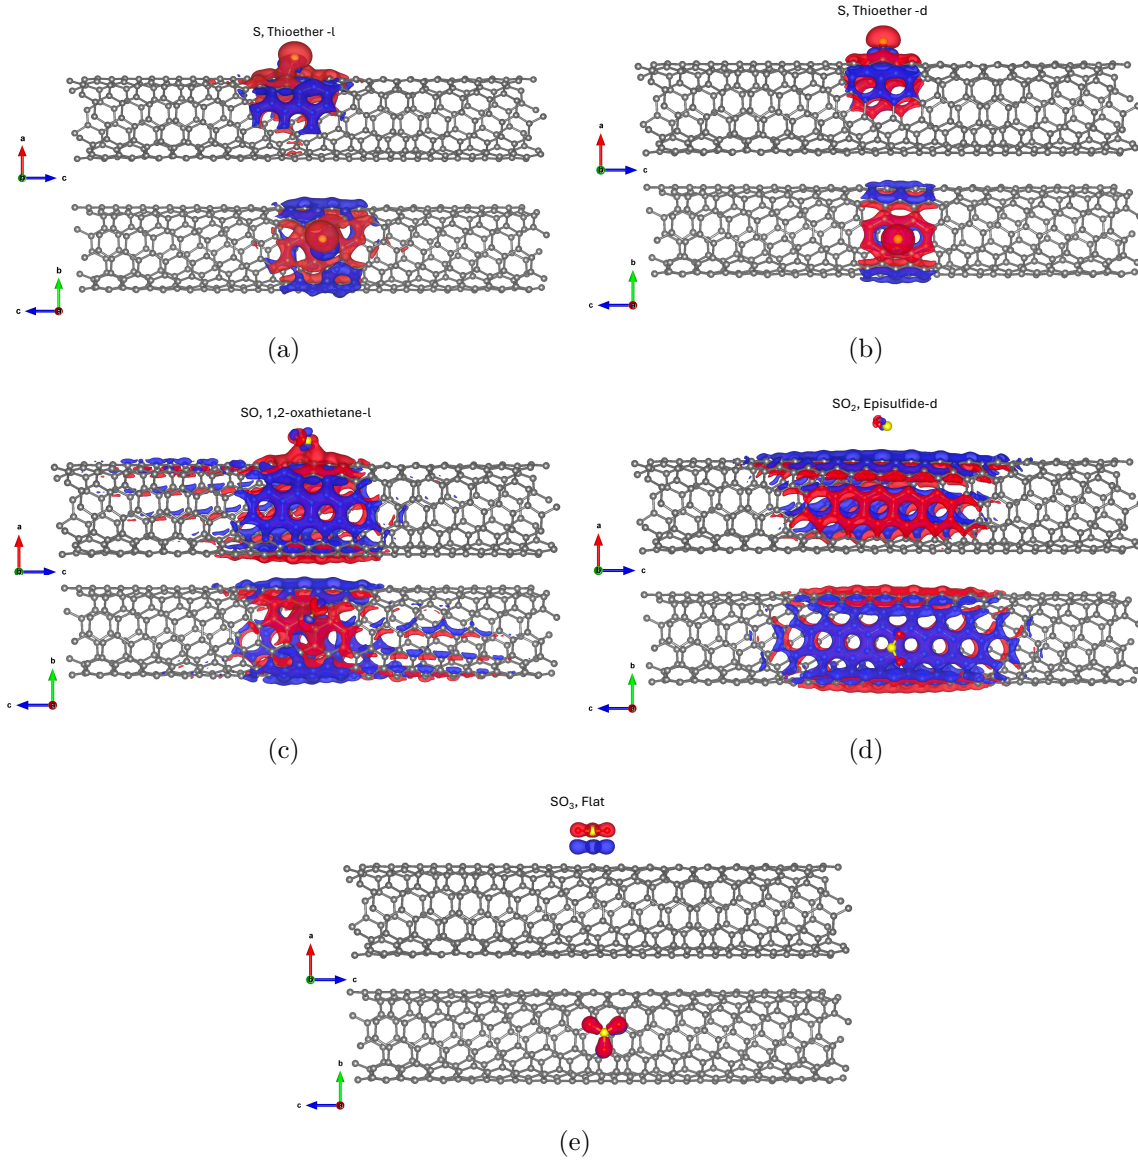

Figure S.2: Electronic charge density differences for the (a) S, thioether-l, (b) S, thioether-d, (c) SO, (d) SO<sub>2</sub> and (e) SO<sub>3</sub> ligands. Each system has been labeled with the ligand orientation, which also corresponds to the band structures in Fig 4 in the main text. The isosurface is chosen such that it captures 40% of the density. The charge differences are colored to show positive electronic difference (red) and negative electronic difference (blue) based on electron density. The charge density differences are shown from two different perspectives: on-top (top) and from the side of the tube (bottom).

Table S.1: Bond lengths, height from the CNT surface ( $h_s$ ) and bond angles for the seven different ligand on the SWCNT and for the  $\text{SO}_2$  and  $\text{SO}_3$  molecules. All distances are given in Å.

| System                         | $R_1 - X$ | $R_2 - X$ | $R_1 - R_2$ | $h_s$ | $S-R_1-R_2$ | $R_1-S-R_2$ | $S-R_2-R_1$ | $O_1-S-O_2$ |
|--------------------------------|-----------|-----------|-------------|-------|-------------|-------------|-------------|-------------|
| S, Episulfide-l                | 1.88      | 1.88      | 1.5         | –     | 66.42       | 47.16       | 66.43       | –           |
| S, Thioether-l                 | 1.88      | 1.88      | 1.50        | –     | 66.42       | 47.15       | 66.43       | –           |
| S, Thioether-d                 | 1.83      | 1.83      | 1.63        | –     | 63.55       | 52.89       | 63.55       | –           |
| SO, 1,2-oxathietane-l          | 2.08      | 2.02      | 1.49        | 1.91  | 66.44       | 42.73       | 70.83       | –           |
| SO,1,2-oxathietane-d           | 2.10      | 2.01      | 1.49        | 1.91  | 65.49       | 42.55       | 71.96       | –           |
| SO <sub>2</sub> , OO-loop-d    | 3.19      | 3.32      | 1.43        | 3.16  | 82.45       | 25.27       | 72.30       | 118.73      |
| SO <sub>2</sub> , Episulfide-d | 3.19      | 3.22      | 1.43        | 3.13  | 78.34       | 25.71       | 75.95       | 118.70      |
| SO <sub>2</sub> , Line-H       | 2.93      | 3.33      | 1.41        | 2.92  | 61.17       | 25.01       | 93.82       | 117.46      |
| SO <sub>3</sub> , flat         | –         | –         | –           | 3.03  | –           | –           | 93.98       | 119.91      |
| CNT-H, Line-H                  | –         | 1.12      | –           | –     | –           | –           | –           | –           |

and SWCNT, indicating chemical bonding. For both  $\text{SO}_2$  and  $\text{SO}_3$ , there is no indicating of charge sharing. For  $\text{SO}_2$ , there is charge redistribution within the tube while for  $\text{SO}_3$ , the charge redistribution is within the molecule only.

### 3 Bandstructure and projected density of states for all bound $\text{SO}_x$ adsorbates

Figure S.5 presents the bandstructures for all seven adsorbates with favorable binding to the CNT. Figures refFig:BSb, c, e, g, and i are presented in Figure 4 of the main text. The conclusions regarding the impact of the other defect configurations on bandstructure is consistent with those presented in the main text.

Figure S.3 presents the projected density of states (PDOS) for all seven adsorbates studied in this work. The PDOS confirms that for S and SO, there is charge mixing between adsorbate and SWCNT with sulfur and oxygen orbital mixing with carbon orbitals (Figure S.3a-d). For unpassivated  $\text{SO}_2$  (Figure S.3 e-f), S and O p-orbital density is only present within the defect band, right below the conduction band. For passivated  $\text{SO}_2$  (Figure S.3g), there is a single peak at the VBM associated with the bound hydrogen and the S/O p-orbitals overlap slightly with the SWCNT conduction band. The  $\text{SO}_3$  system shown in (h) also show overlap between the S/O p-orbital densities with the CNT conduction band, which we attribute to possible artificial mixing of the bands due to the delocalization of error of DFT.

Figure S.4 presents the band splitting in the valence (Fig. 4(a)) and conduction (Fig. 4(b)) bands for the pristine and five doped systems shown in Figure 4 in the main text along the Brillouin Zone path. Both plots show that there is significant band splitting in the presence of the S and SO adsorbates in the valence and conduction bands, while the  $\text{SO}_2$  adsorbate show very little band splitting and  $\text{SO}_3$  only shows splitting in the conduction band.

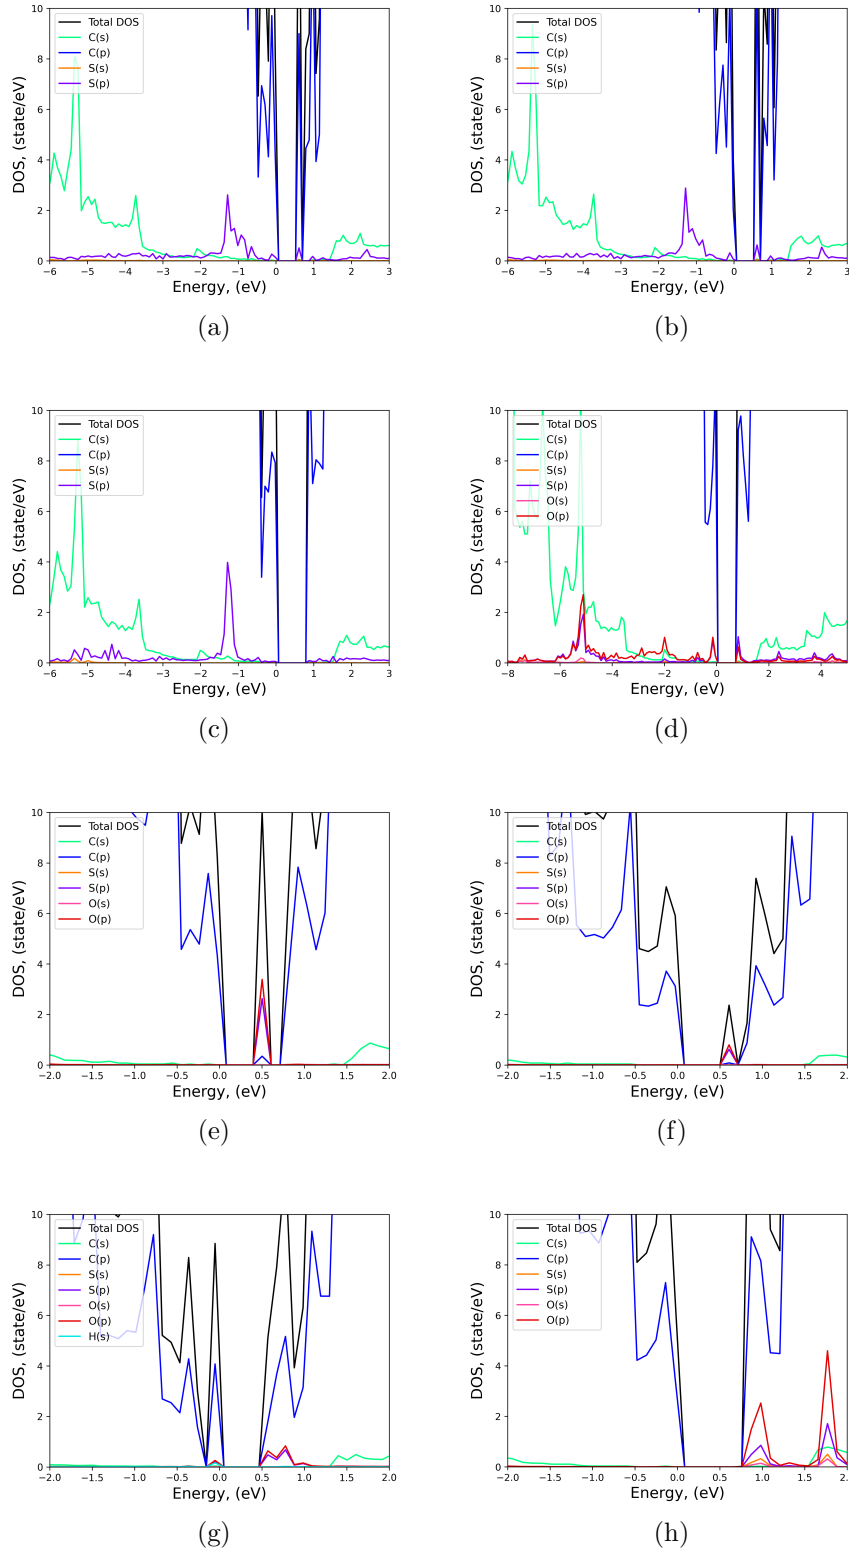

Figure S.3: Projected density of states (PDOS) for (a) S, episulfide-l, (b) S, thioether-l, (c) S, thioether-d, (d) SO, 1,2-oxathietane-l, (e) SO<sub>2</sub>, OO-loop-d, (f) SO<sub>2</sub>, episulfide-l, (g) SO<sub>2</sub>, line-H, and (h) SO<sub>3</sub>, flat. All graphs have been zeroed to the valence band maximum (VBM).

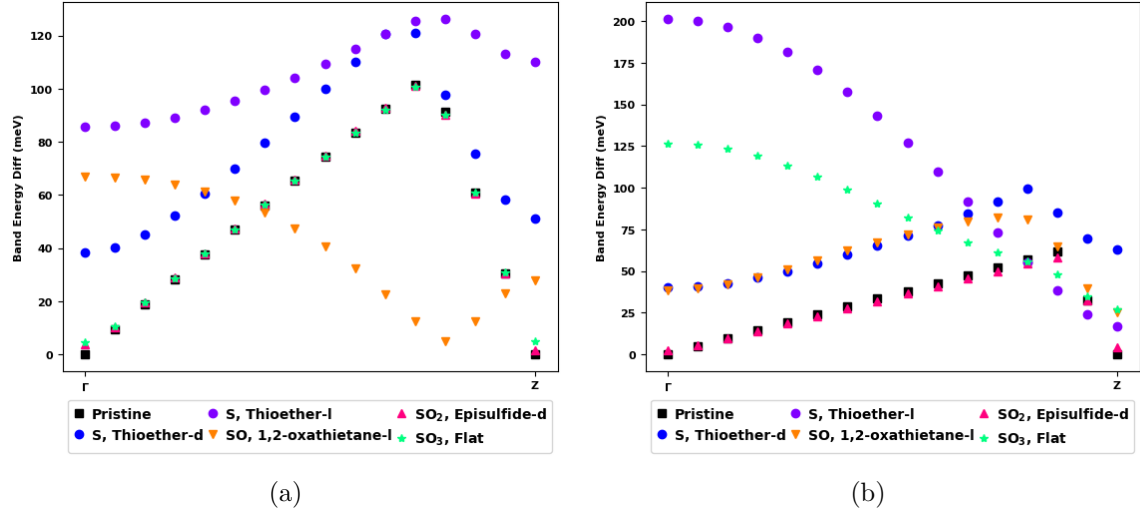

Figure S.4: Band energy difference between the (a) valence band max (VBM) and VBM-1 bands and the (b) conduction band min (CBM) and CBM+1 bands of the SWCNT for the pristine system compared to the five different adsorbates shown in Figure 4 in the main text. All energy differences are shown as absolute values.

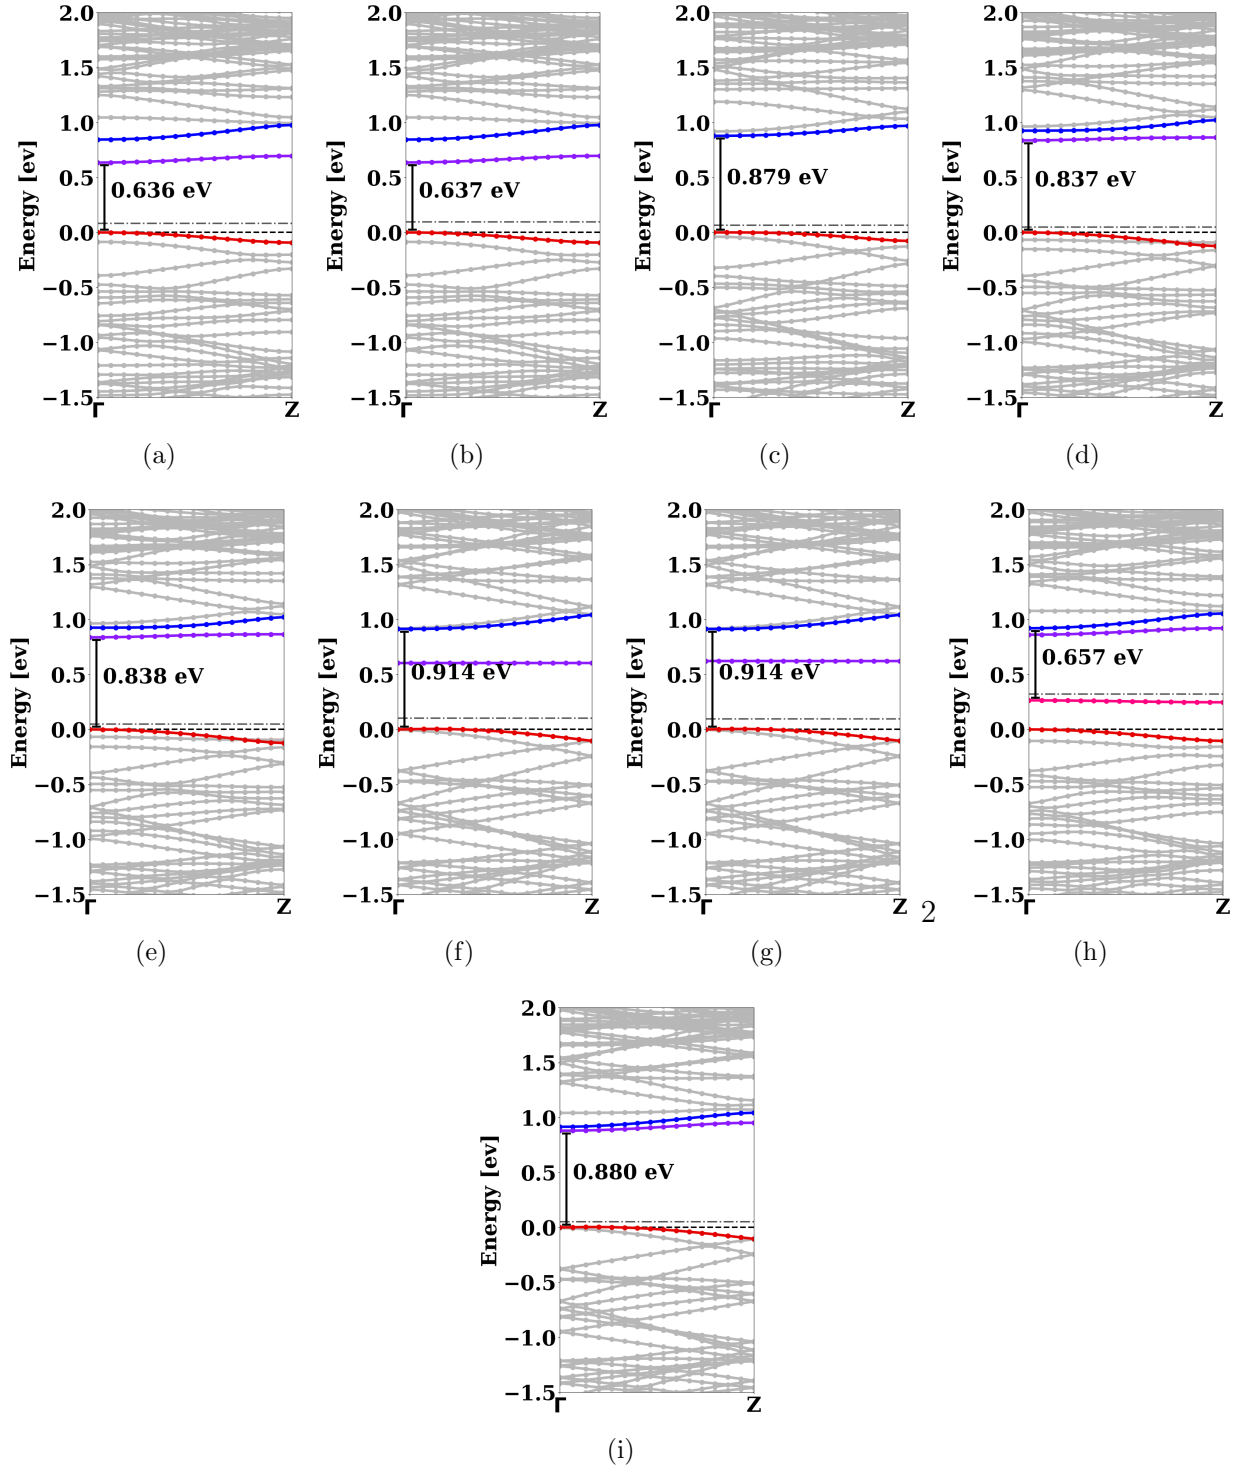

Figure S.5: Band structures for (a) S, episulfide-l, (b) S, thioether-l, (c) S, thioether-d, (d) SO, 1,2-oxathietane-d, (e) SO, 1,2-oxathietane-l, (f) SO<sub>2</sub>, OO-loop-d, (g) SO<sub>2</sub>, episulfide-l, (h) SO<sub>2</sub>, line-H, and (i) SO<sub>3</sub>, flat. Occupied pristine-like valence bands and unoccupied conduction bands are shown in red and blue, respectively, while unoccupied states localized on the defect are in purple. The gray dash-dot line on each band structure represents the Fermi energy level. All plots are shifted such that the top of the pristine-like valence band is at zero at  $\mathbf{k} = 0$  (indicated by black dash line).
